# Supplementary material for: A Diffusion-Based Framework for Terrain-Aware Remote Sensing Image Reconstruction
Source: arXiv:2504.12112 source file (2025-04-16)
Supplement: Supplementary file 1 [file X_suppl.tex]

\clearpage
\setcounter{page}{1}
\setcounter{section}{0}
\setcounter{table}{0}
\setcounter{figure}{0}

% \maketitlesupplementary

% % table:data_info - appendix
% \begin{table*}
%     \centering
%     \caption{Data Information. Notes: cloud cover $\leq$ 1\%. The regions were randomly selected, but it was required to ensure that there were available Landsat-8 images within these areas.}
%     \begin{tabular}{ccccc}
%         \hline
%         \textbf{No.} & \textbf{Country / Region} & \textbf{Coordinates (Center Point)} & \textbf{Latitude Range} & \textbf{Longitude Range} \\
%         \hline
%         01 & New Zealand - Near Christchurch & (-24.75, 65.25) & 65.0 - 65.5 & -25.0 - -24.5 \\
%         02 & Namibia - Near Windhoek & (15.25, -21.75) & -22.0 - -21.5 & 15.0 - 15.5 \\
%         03 & China - Near Xi'an, Shaanxi Province & (108.75, 34.25) & 34.0 - 34.5 & 108.5 - 109.0 \\
%         04 & United States - California & (-120.25, 35.25) & 35.0 - 35.5 & -120.5 - -120.0 \\
%         05 & Italy - Northern Region & (10.25, 45.25) & 45.0 - 45.5 & 10.0 - 10.5 \\
%         06 & Japan - Near Tokyo & (139.75, 35.75) & 35.5 - 36.0 & 139.5 - 140.0 \\
%         07 & France - Near Paris & (2.25, 48.75) & 48.5 - 49.0 & 2.0 - 2.5 \\
%         08 & United States - Near Seattle, Washington & (20.25, 64.25) & 64.0 - 64.5 & 20.0 - 20.5 \\
%         09 & Argentina - Buenos Aires & (-58.25, -34.25) & -34.5 - -34.0 & -58.5 - -58.0 \\
%         10 & Australia - Near Melbourne & (144.75, -37.25) & -37.5 - -37.0 & 144.5 - 145.0 \\
%         \hline
%     \end{tabular}
%     \label{table:data_info}
% \end{table*}

\section{Landsat Dataset}
\label{appendix_geecode}

The data used in this study, including the Digital Elevation Model (DEM) and Landsat 8 imagery, were sourced from the Google Earth Engine (GEE) platform. GEE provides a vast repository of satellite imagery and geospatial datasets, which can be accessed programmatically using its API. Below is the code used for downloading the selected data for the study. This script extracts the required images, applies the necessary filters, and prepares the data for analysis. This code filters and downloads Landsat 8 imagery with less than 1\% cloud cover and the corresponding DEM data for the specified region of interest (ROI). The data is then exported to Google Drive for further analysis. We selected 10 regions, with the range of the ROIs shown in Table \ref{table:data_info}, and their spatial distribution illustrated in Fig. \ref{fig:site_map}.

\lstdefinelanguage{JavaScript}{
  morekeywords={typeof, new, true, false, catch, function, return, null, catch, switch, var, let, const, if, in, while, do, else, case, break, for, try, throw, async, await},
  morestring=[b]',
  morestring=[b]",
  morecomment=[l]{//},
  morecomment=[s]{/*}{*/},
  keywordstyle=\color{blue}\bfseries,
  stringstyle=\color{red},
  commentstyle=\color{gray},
  identifierstyle=\color{black},
  sensitive=true
}

\lstset{
    language=JavaScript,
    basicstyle=\ttfamily\footnotesize,
    numbers=left,
    numberstyle=\tiny\color{gray},
    stepnumber=1,
    breaklines=true,
    frame=single,
    captionpos=b,
    keywordstyle=\color{blue}\bfseries,
    stringstyle=\color{darkred},
    commentstyle=\color{gray}\itshape,
    identifierstyle=\color{black},
    xleftmargin=20pt,  % 调整左侧边距
    % xrightmargin=10pt  % 调整右侧边距
}

\begin{lstlisting}[language=JavaScript, caption={Landsat Dataset Download Code}]

// Using Google Earth Engine JavaScript API to retrieve DEM and Landsat 8 imagery for specific regions

// Define Areas of Interest (AOI) with corresponding country/region names

// Region 1: Near Christchurch, New Zealand
var region1 = ee.Geometry.Polygon([
  [-25.0, 65.0], [-24.5, 65.0], [-24.5, 65.5], [-25.0, 65.5], [-25.0, 65.0]
]);

// Region 2: Near Windhoek, Namibia
var region2 = ee.Geometry.Polygon([
  [15.0, -22.0], [15.5, -22.0], [15.5, -21.5], [15.0, -21.5], [15.0, -22.0]
]);

// Region 3: Near Xi'an, Shaanxi Province, China
var region3 = ee.Geometry.Polygon([
  [108.5, 34.0], [109.0, 34.0], [109.0, 34.5], [108.5, 34.5], [108.5, 34.0]
]);

// Region 4: California, United States
var region4 = ee.Geometry.Polygon([
  [-120.5, 35.0], [-120.0, 35.0], [-120.0, 35.5], [-120.5, 35.5], [-120.5, 35.0]
]);

// Region 5: Northern Italy
var region5 = ee.Geometry.Polygon([
  [10.0, 45.0], [10.5, 45.0], [10.5, 45.5], [10.0, 45.5], [10.0, 45.0]
]);

// Region 6: Near Tokyo, Japan
var region6 = ee.Geometry.Polygon([
  [139.5, 35.5], [140.0, 35.5], [140.0, 36.0], [139.5, 36.0]
]);

// Region 7: Near Paris, France
var region7 = ee.Geometry.Polygon([
  [2.0, 48.5], [2.5, 48.5], [2.5, 49.0], [2.0, 49.0]
]);

// Region 8: Near Seattle, Washington, United States
var region8 = ee.Geometry.Polygon([
  [20.0, 64.0], [20.5, 64.0], [20.5, 64.5], [20.0, 64.5]
]);

// Region 9: Buenos Aires, Argentina
var region9 = ee.Geometry.Polygon([
  [-58.5, -34.5], [-58.0, -34.5], [-58.0, -34.0], [-58.5, -34.0]
]);

// Region 10: Near Melbourne, Australia
var region10 = ee.Geometry.Polygon([
  [144.5, -37.5], [145.0, -37.5], [145.0, -37.0], [144.5, -37.0]
]);

// Using Region 8 as an example
var region = region8;

// Retrieve SRTM DEM data and clip it to the Area of Interest (AOI)
var srtm = ee.Image('USGS/SRTMGL1_003').clip(region).toFloat();

// Retrieve Landsat 8 imagery with cloud cover less than 1%, filtered by date and region, including all bands
var landsat = ee.ImageCollection('LANDSAT/LC08/C02/T1_TOA')
  .filterBounds(region)
  .filterDate('2013-01-01', '2022-12-31')
  .filter(ee.Filter.lt('CLOUD_COVER', 1))
  .median()
  .clip(region)
  .toFloat();

// Visualization settings
var srtmVis = {min: 0, max: 3000, palette: ['#440154', '#3b528b', '#21908d', '#5ec962', '#fde725']};
var landsatVis = {bands: ['B4', 'B3', 'B2'], min: 0, max: 3000, gamma: 1.4, palette: ['#8c510a', '#bf812d', '#dfc27d', '#f6e8c3', '#c7eae5', '#80cdc1', '#35978f', '#01665e']};

// Add SRTM and Landsat 8 imagery to the map
Map.centerObject(region, 10);
Map.addLayer(srtm, srtmVis, 'SRTM DEM');
Map.addLayer(landsat, landsatVis, 'Landsat 8');

// Export SRTM DEM data to Google Drive
Export.image.toDrive({
  image: srtm,
  description: 'srtm_dem_region8',
  folder: 'output_gee_data',
  scale: 30,
  region: region,
  fileFormat: 'GeoTIFF'
});

// Export Landsat 8 imagery to Google Drive
Export.image.toDrive({
  image: landsat,
  description: 'landsat8_image_region8',
  folder: 'output_gee_data',
  scale: 30,
  region: region,
  fileFormat: 'GeoTIFF'
});

// Export AOI vector shapefile to Google Drive
Export.table.toDrive({
  collection: ee.FeatureCollection(ee.Feature(region)),
  description: 'aoi_shapefile_region8',
  folder: 'output_gee_data',
  fileFormat: 'SHP'
});

\end{lstlisting}

\section{Figures}
% The selected regions for Landsat imagery in Task-1 is shown in Figure \ref{fig:site_map}.

The structure of VGG-Adapter is shown in Figure \ref{fig_vgg19}.

\begin{figure*}[!ht]
    \centering
    \includegraphics[width=1.0\linewidth]{figs/vgg19.pdf}
    \caption{VGG-Adapter Module Architecture. The VGG-Adapter module is designed to reduce distribution shifts and improve consistency in remote sensing image reconstruction. Built upon the VGG-19 network, it extracts multi-scale feature representations from convolutional layers ($conv1_1, conv2_1, conv3_1, conv4_1, conv5_1$) and aligns them with the reference image. The module incorporates distribution loss to minimize feature discrepancies, ensuring improved stability and perceptual quality in generated images.}
    \label{fig_vgg19}
\end{figure*}
